# Supplementary material for: Efficient and Consistent Robust Time Series Analysis
Source: arXiv:1607.00146 source file (2016-07-01)
Supplement: Supplementary file 1 [file appendix.tex]

%\input{app_inn}

%%% Local Variables:
%%% mode: latex
%%% TeX-master: "robust_ts"
%%% End:
